# Supplementary material for: Rovibrational-Specific QCT and Master Equation Study on $\text{N}_2(\text{X}^1\Sigma_g^+)$+$\text{O}({}^3\text{P})$ and $\text{NO}(\text{X}^2\Pi)$+$\text{N}({}^4\text{S})$ Systems in High-Energy Collisions
Source: arXiv:2111.01751 source file (2021-11-02)
Supplement: Supplementary file 1 [file SupplementaryMaterial.pdf]

Supplementary Material:  
Rovibrational-Specific QCT and Master Equation Study on  
 $\text{N}_2(\text{X}^1\Sigma_g^+) + \text{O}(\text{}^3\text{P})$  and  $\text{NO}(\text{X}^2\Pi) + \text{N}(\text{}^4\text{S})$  Systems in  
High-Energy Collisions

Sung Min Jo,<sup>1</sup> Simone Venturi,<sup>1</sup> Maitreyee P. Sharma,<sup>1</sup> Alessandro Munafò,<sup>1</sup>  
Marco Panesi<sup>1,a)</sup>

<sup>1</sup>Center for Hypersonics and Entry Systems Studies (CHESS),  
University of Illinois at Urbana-Champaign, Urbana, IL 61801, USA

<sup>a)</sup>Electronic mail: mpanesi@illinois.edu

November 2, 2021

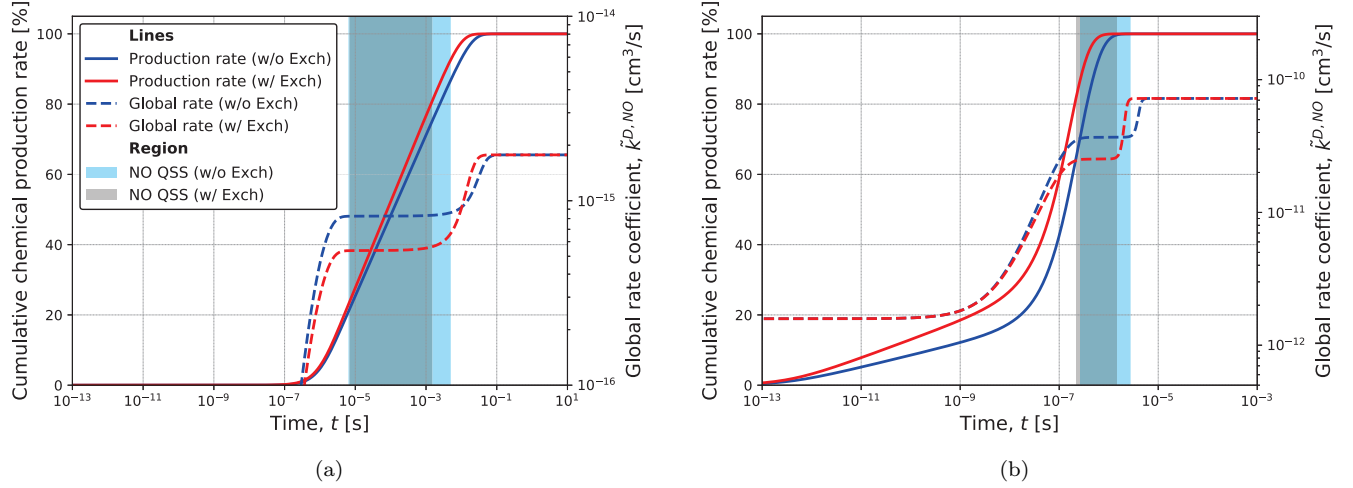

**Figure S1:** Time-cumulative chemical production and global dissociation rate distributions for the NO+N system (heterogeneous exchange process excluded). The solid lines indicate the chemical production rates, while the dashed lines represent the global dissociation rate coefficients. The shaded regions indicate the QSS periods of NO. (a)  $T=5000$  K, (b)  $T=20000$  K. The figures share the plot legend.

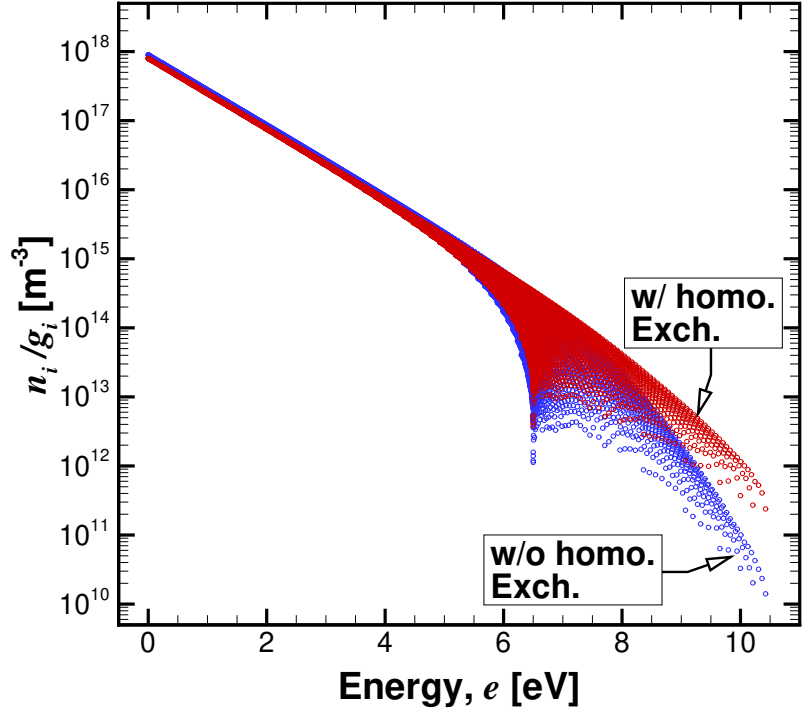

**Figure S2:** Comparison of the QSS rovibrational distributions of NO at  $T=10\,000\text{ K}$  with and without homogeneous exchange kinetics. The initial mole fraction is set to  $\chi_{\text{NO}}=\chi_{\text{N}}=0.5$ .

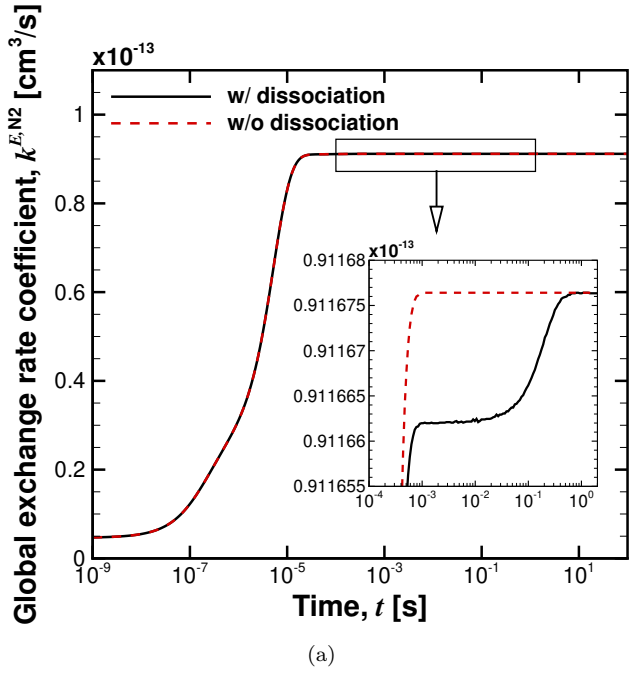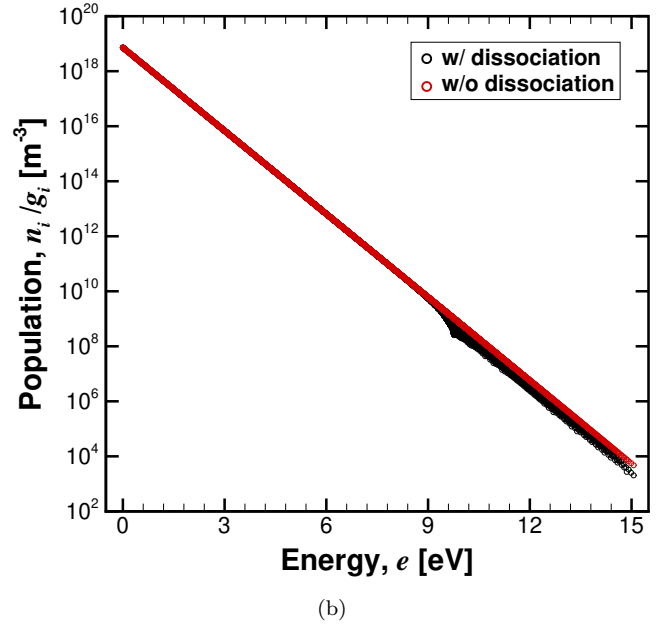

**Figure S3:** Comparisons of (a) the global rate coefficient for  $\text{N}_2+\text{O} \rightarrow \text{NO}+\text{N}$ , (b) the corresponding rovibrational distributions of  $\text{N}_2$  at  $t=8 \times 10^{-4}\text{ s}$  at  $T=5000\text{ K}$  for cases that the system has dissociation kinetics and not. The initial mole fraction was set to  $\chi_{\text{N}_2}=\chi_{\text{O}}=0.5$ .

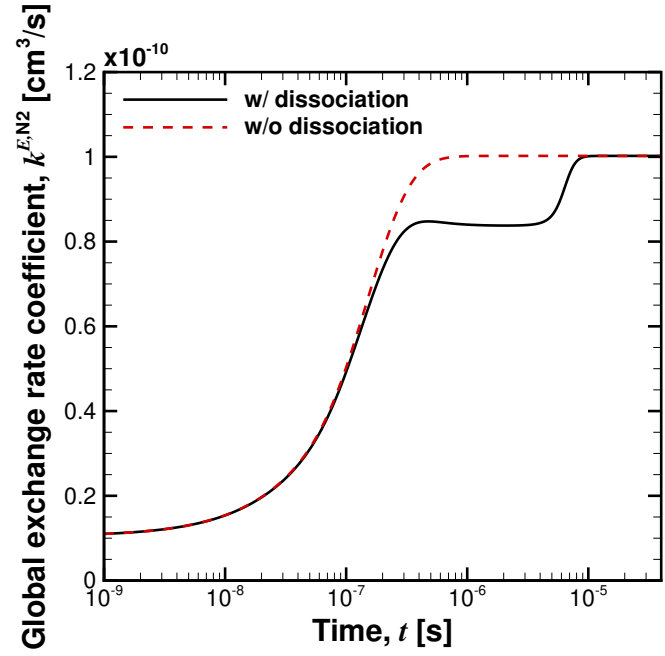

(a)

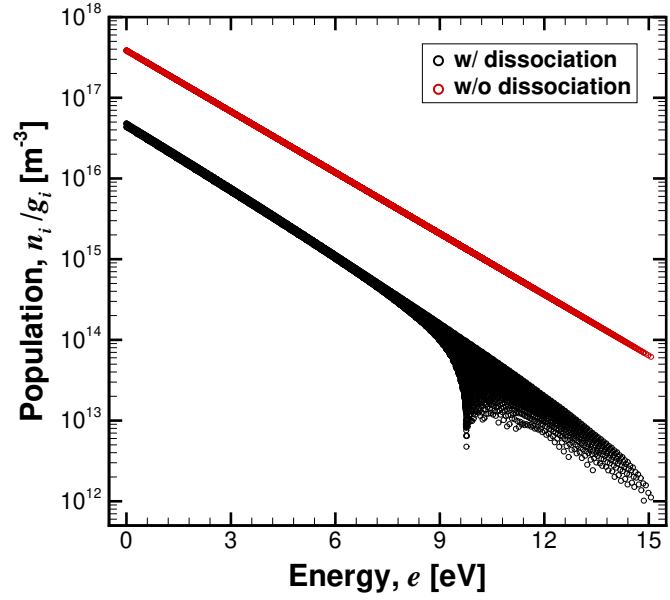

(b)

**Figure S4:** Comparisons of (a) the global rate coefficient for  $\text{N}_2 + \text{O} \rightarrow \text{NO} + \text{N}$ , (b) the corresponding rovibrational distributions of  $\text{N}_2$  at  $t=1 \times 10^{-6}$  s at  $T=20\,000$  K for cases that the system has dissociation kinetics and not. The initial mole fraction was set to  $\chi_{\text{N}_2}=\chi_{\text{O}}=0.5$ .
